# Supplementary material for: Variational Bayes for high-dimensional proportional hazards models with applications within gene expression
Source: arXiv:2112.10270 source file (2022-07-05)

(b)

 $l_1$ -error $l_1$ -error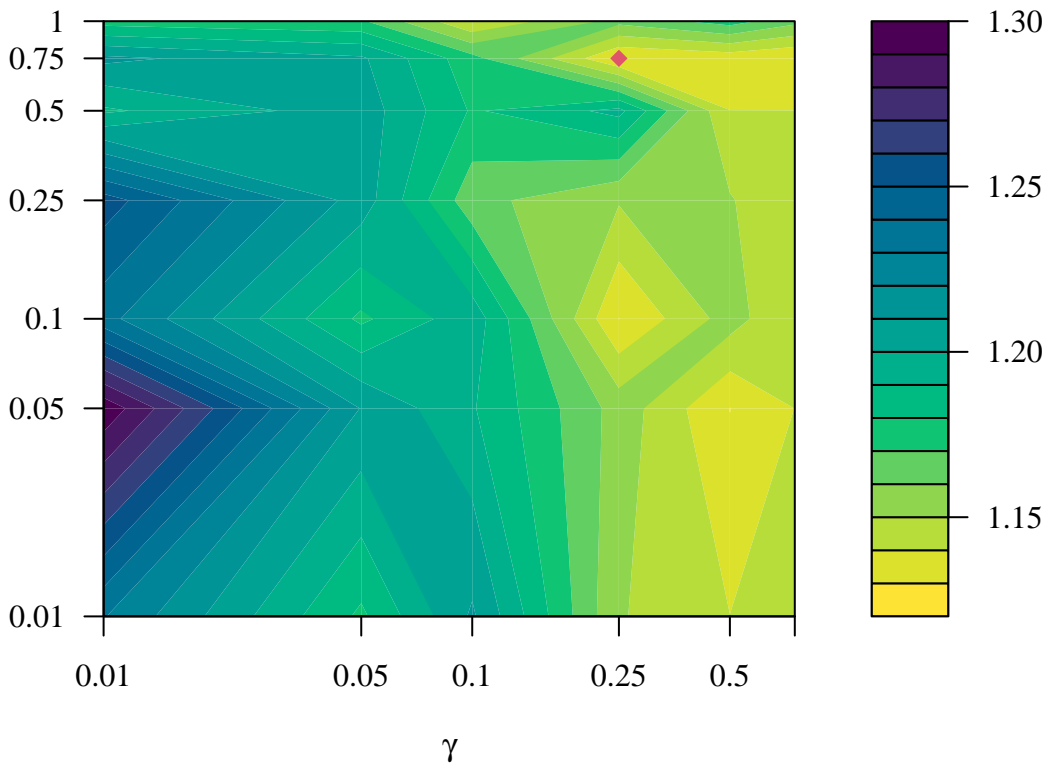

Supplement: Supplementary file 2 [file sensitivity_s_g_2_2.pdf]
