# Supplementary material for: Variational Bayes for high-dimensional proportional hazards models with applications within gene expression
Source: arXiv:2112.10270 source file (2022-07-05)

(d)

FDR

FDR

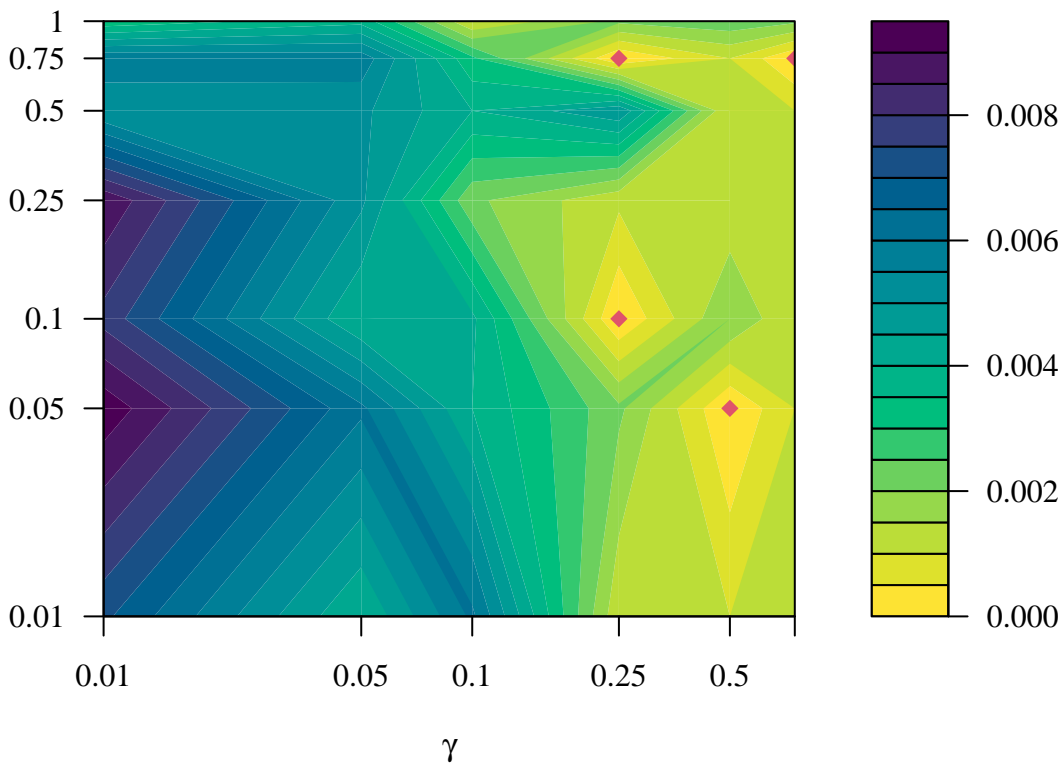

Supplement: Supplementary file 4 [file sensitivity_s_g_2_4.pdf]
