# Supplementary material for: Variational Bayes for high-dimensional proportional hazards models with applications within gene expression
Source: arXiv:2112.10270 source file (2022-07-05)

(f)

Time (s)

Time (s)

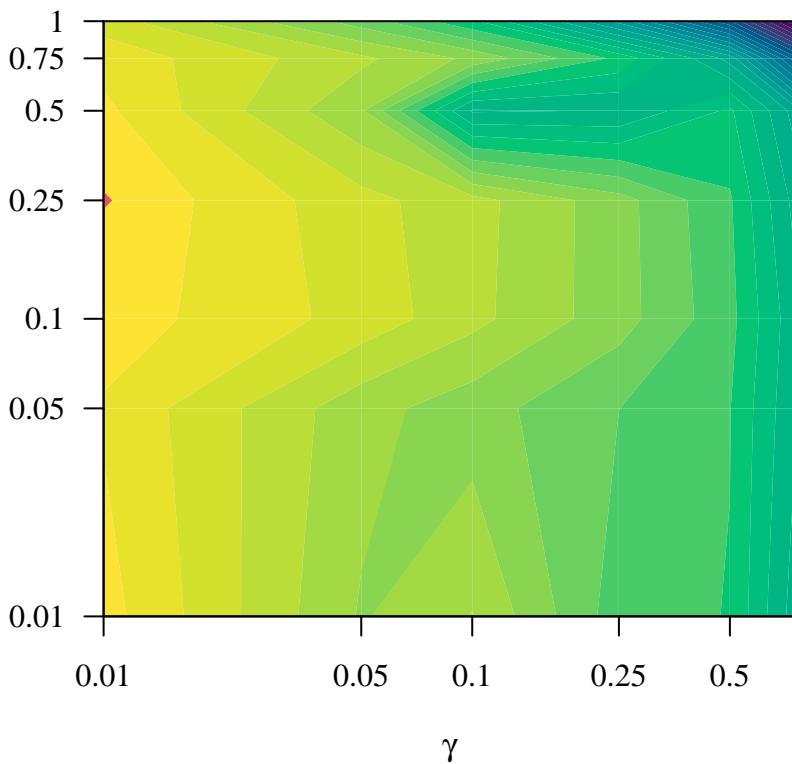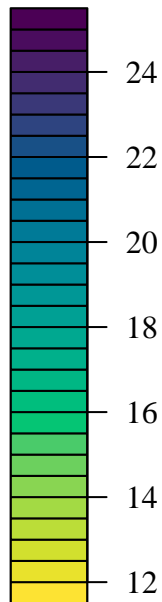

Supplement: Supplementary file 6 [file sensitivity_s_g_2_6.pdf]
